# Supplementary material for: Generating Leakage-Free Benchmarks for Robust RAG Evaluation
Source: arXiv:2605.08838 source file (2026-05-09)
Supplement: Supplementary file 1 [file 6appendix.tex]

\section{Appendix}
